# Supplementary material for: The addition of temporal neighborhood makes the logic of prefixes and sub-intervals EXPSPACE-complete
Source: arXiv:2202.07881 source file (2024-03-21)
Supplement: Supplementary file 1 [file appendixHardness.tex]

%!TEX root = ./main.tex

\section{\expspace-hardness of
\texorpdfstring{$\mathsf{BDA}_{hom}$}\ via Tiling }\label{appendix:hardness}

In this section we prove that the satisfiability
problem for $\mathsf{BDA}_{hom}$ interpreted over
finite linear orders is \expspace-hard using a suitable tiling problem. The result
is obtained by a reduction from the \emph{exponential-corridor
tiling problem}, which is known to be \expspace-complete
\cite{van1997convenience}. Such a problem can be stated
as follows.

\begin{problem}\label{prob:exptiling}
Given a tuple $\cT = (T, \tileH,\tileV,C)$ where $T, C \in \bbN$ ($C$ is expressed in binary),
and $\tileH,\tileV\subseteq \{0, \ldots, T\}\times \{0, \ldots, T\}$,
the exponential-corridor
tiling problem consists of
determining whether or not there exists a function
$tile: \bbN \times \{0,\ldots, C\}\rightarrow \{0, \ldots, T\}$ such that:
\begin{compactenum}
\item\label{prob:exptiling:topbot} for every $x \in \bbN$ we have
 $tile(x,0) = 0$ and $tile(x,C)=T$;
\item\label{prob:exptiling:hor} for every $x \in \bbN$
and every $0 \leq y \leq C$ 
we have $(tile(x,y),tile(x+1,y)) \in \tileH$;
\item\label{prob:exptiling:ver} for every $x \in \bbN$
and every $0 \leq y < C$ 
we have $(tile(x,y),tile(x,y+1)) \in \tileV$.
\end{compactenum}
\end{problem}

\vspace{-0.0cm}

\noindent The following classical result 
will be exploited to prove the main goal of this section.

\vspace{-0.0cm}

\begin{theorem}\label{thm:tilingexpspacehard}\cite{van1997convenience}
The exponential-corridor
tiling problem is EXPSPACE-hard.
\end{theorem}

\vspace{-0.0cm}

To define a reduction 
from Problem~\ref{prob:exptiling} to  the finite satisfiability of
$\mathsf{BDA}_{hom}$ we have to face the problem that
formulas of $\mathsf{BDA}_{hom}$ are interpreted over finite domains, whereas the $tile$ functions ranges over an infinite domain. Roughly speaking, we will solve Problem~\ref{prob:exptiling} by means of an infinite ``unfolding'' of  a finite portion of the tiling space that can be  encoded by a (finite) model for a suitable $\mathsf{BDA}_{hom}$ formula. 
The following result is crucial to that purpose.

\vspace{-0.0cm}

\begin{lemma}\label{lem:finitecorridor}
Given an instance $\cT = (T, \tileH,\tileV,C)$ of Problem~\ref{lem:finitecorridor}
we have that $\cT$ is a positive instance if and only if there 
exists a function $tile:\bbN \times \{0,\ldots, C\}\rightarrow 
\{0, \ldots, T\}$ that fulfills conditions \ref{prob:exptiling:topbot},
\ref{prob:exptiling:hor}, and \ref{prob:exptiling:ver} of 
Problem~\ref{prob:exptiling} together with the following one:
\vspace{-0.0cm}
\begin{compactenum}
\item[(4)] 
there exist $prefix\in \bbN$ and $period\in\bbN^+$ 
s.t. for every $x \geq prefix$ and every $0\leq y\leq C$  we have
$tile(x,y)=tile(x+period,y)$.
\end{compactenum}
\end{lemma}
\vspace{-0.0cm}

The proof of Lemma~\ref{lem:finitecorridor} is straightforward
and omitted. Lemma~\ref{lem:finitecorridor} allows us to 
bound the search space for the existence of the function $tile$
to a finitely representable function $\otile:
\{0,\ldots, prefix, \ldots, prefix + period \} \rightarrow \{0, \ldots, T\}$
for some $prefix \geq 0$ and $period >0$. Function $\otile$
witnesses that $\cT$ is a positive instance of 
Problem~\ref{prob:exptiling} if it satisfies conditions \ref{prob:exptiling:topbot}, \ref{prob:exptiling:hor}, and \ref{prob:exptiling:ver} restricted to
$(x,y)\in \bbN \times \{0, \ldots, C\}$ with $x < prefix + period$
plus the condition that $\otile(prefix, y)=\otile(prefix+period,y)$
for every $y \in\{0, \ldots, C\}$.

Given an instance $\cT = (T, \tileH,\tileV,C)$ of 
Problem~\ref{prob:exptiling} we
provide  a $\mathsf{BDA}_{hom}$ formula $\varphi_{\cT}$ 
that is satisfiable over finite models if and  only
if there exists a function $\otile$ that satisfies the
aforementioned properties and thus, by Lemma~\ref{lem:finitecorridor},
if and only if $\cT$ is a positive instance of Problem~\ref{prob:exptiling}.
In the proposed encoding we force each point of the model to 
represent exactly one tile. This is done by exploiting $T + 1$
propositional variables $t_0, \ldots, t_T$, called \emph{tile variables}, 
constrained by the following formulas\footnote{In the encoding we will make extensive use of the
``global'' operator whose semantics was introduced in Section~\ref{sec:hardness}.}:

%\vspace{-1cm}

\[\begin{array}{l}
\psi_\exists= \hsA\left(\pi \rightarrow \bigvee\limits_{i=0}^T t_i
\right), \mbox{ given a point in the model \emph{at least} 
one tile variable holds over it;} \\ \\
\arraycellcomment{\psi_!=\hsA \left( \bigwedge\limits_{i=0}^T
\left(t_i \wedge \pi \rightarrow \left(\bigwedge\limits_{j=0, j \neq i}^T
  \neg t_j  \right)
 \right)\right),}{8cm}{given a point in the model \emph{at most}
 one tile variable holds over it (i.e., mutual exclusion).}
 \end{array}\]

%\vspace{-0.0cm}

Let us assume w.l.o.g. that $C= 2^c - 1$ for some $c \in \bbN$. Then, we
associate to each model point a number in $\{0, \ldots, C\}$ by 
a binary encoding via $c$-propositional variables
$b_1,\ldots, b_c$, where $b_1$ is the most significant bit. Formally, 
given a model $\bfM = (N, \cV)$ and a point we define a function with

$bit_{\cV}: \{0, \ldots, N\}\times \{b_1,\ldots,b_c \}
\rightarrow \{0,1\}$ where $bit_{\cV} (n, b_i) = \left\{\begin{array}{ll}
1 & \mbox{if $b_i \in \cV([n,n])$}\\
0 & \mbox{otherwise}
\end{array}\right.$. 

For the sake of brevity, we denote with $\oy_n$ the natural number whose $c$-bit 
length binary encoding is $bit_{\cV}(n,b_1)\ldots bit_{\cV}(n,b_c)$. We encode the domain of a general
function $\otile:\{0,\ldots, prefix, \ldots, prefix + period \} \rightarrow \{0, \ldots, T\}$ 
into a finite model $\bfM = (N, \cV)$ by enumerating all the points of the grid
$\{0, \ldots,\allowbreak prefix + suffix \} \times \{0, \ldots, C\}$ along the timepoints
$\{0, \ldots, N\}$ of the model in a lexicographical order. 
The formula  $\psi_{\otile} = \psi_{\exists} \wedge \psi_! \wedge \psi_{boundaries} \wedge \psi_\uparrow$ is used to force such constraint
where $\psi_{boundaries}$ and $\psi_\uparrow$ are formulas defined as follows:

\vspace{-0.3cm}

\[\begin{array}{l}
\arraycellcomment{\psi_{boundaries} =
\hsEB\left(\pi \wedge \bigwedge\limits_{i=1}^c \neg b_i\right)
\wedge \hsAA\left(\bigwedge\limits_{i=1}^c b_i\right), }
{7.3cm}
{ every model $\bfM = (N, \cV)$ for $\psi_{boundaries}$  satisfies $\oy_0=0$ and $\oy_N = C$;}\\ \\
%\end{array}\]
%\[\begin{array}{l}
 \arraycellcomment{
 \psi_{\uparrow} =
 \hsA\left( \hsAB \pi \rightarrow
 \left(\bigwedge\limits_{i=1}^c \hsEB b_i  \wedge \left(
 \hsAA \bot  \vee \bigwedge\limits_{i=1}^c \hsEA (\pi \rightarrow \neg b_i)
 \right)\right) \vee \psi^1_{+}  \right),
 }{3.6cm}{for every  $n \in \{0, \ldots, N\}$
 if $\oy_n=C$ then either $n=N$ or $\oy_{n + 1}= 0$,
 if $\oy_n <N $ then $\oy_{n+1} = \oy_{n} +1$; }\\
\\ 
\arraycellcomment{
 \psi^i_{+} = \begin{array}{l}
 (\hsEB b_i \rightarrow \hsEA (\pi \wedge \neg b_i)\wedge 
 \psi^{i+1}_{+})
 \wedge \\
 (\hsEB \neg b_i \rightarrow \hsEA b_i \wedge 
 \psi^{i+1}_{=})\end{array},
 }{7.9cm}{
 formula $\psi^i_{+}$ encodes the bit-wise
 increment for every bit $b_i$ with 
 $i\in \{1, \ldots, c - 1\}$; $\psi^1_{+}$
 is triggered by $\psi_{\uparrow}$
 on every interval $[n, n+1]$ with $\oy_{n} < C$;}\\ \\
 \arraycellcomment{
 \psi^c_{+} = 
 \neg \hsEB b_i \wedge \hsEA b_i,
 }{11.2cm}{
 formula $\psi^c_{+}$ encodes the bit-wise
 increment for the bit $b_c$; it is triggered
 by $\psi^{c-1}_{+}$ on every interval 
 $[n, n+1]$ for which $bit_{\cV}(n,b_i)=1$
 for every $1\leq i < c$;  let us notice that it does not propagate 
 and it handles overflows by creating a contradiction; }
 \\
\end{array}
\]
\[
\begin{array}{l}

%\end{array}\]
%\[\begin{array}{l}
 \arraycellcomment{
 \psi^i_{=} = \neg \pi \wedge  
 \bigwedge\limits_{j=i}^{j=c} \left(
 \hsEB( \pi \wedge b_i) \leftrightarrow \hsEA (\pi \wedge b_i)
 \right),
 }{7.4cm}
 { formula $\psi^i_{=}$ holds over an interval 
 $[n,n']$ if and only if $n<n'$ and
 $bit_{\cV}(n,b_j)=bit_{\cV}(n',b_j)$ for every $i\leq j \leq c$; } 
 \vspace{-0.0cm}
  \end{array}\]
%\vspace{-0.5cm}
%\[\begin{array}{l}
% \mbox{\begin{tabular}{p{15.5cm}}
 Note that if $\psi^1_{=}$ holds over $[n,n']$ then $\oy_n = \oy_{n'}$. Formula $\psi^i_{=}$ is used for guaranteeing the correct bitwise increment 
 in formulas $\psi^i_{+}$, moreover it will be used in the following for correctly identifying tiles which are in the $\tileH$ relation.\\ \\
% \end{tabular}
% }
% \end{array}\]
%
%\vspace{-0.5cm}
%
%
 \noindent It is worth noticing 
 that any model $\bfM = (N, \cV)$  that satisfies 
 $\psi_{\otile} = \psi_{\exists} \wedge \psi_! \wedge \psi_{boundaries}
 \wedge \psi_\uparrow$  fulfills some properties. First of all,
 the interplay  between $\psi_{boundaries}$ and  $\psi_\uparrow$ 
 guarantees that $N$ is a multiple of $(C+1)$ and thus, 
 for suitably chosen $prefix$ and $suffix$, we can associate each point  
 $(x, y) \in \{0, \ldots,\allowbreak prefix + suffix \} \times 
 \{0, \ldots, C\}$ to a point $n \in \{0, \ldots, N\}$ by means of a 
 bijection $map: \{0, \ldots,\allowbreak prefix + suffix \} \times 
 \{0, \ldots, C\}\rightarrow \{0, \ldots, N\}$ defined as
  $map(x,y)=x\cdot (C+1) 
 + y$ (i.e.,  $map^{-1}(n)= (\lfloor \frac{n}{C + 1} \rfloor, n\ \mbox{\%}\ C  )$
 where \% is the integer remainder operation). Moreover,  
 let us observe that for every element $(x, y)$ in the grid, we have 
 that $x$ is just implicitly encoded in the model by $map(x,y)$ 
 (i.e., $x =\lfloor \frac{map(x,y)}{C + 1} \rfloor$), while 
 $y$ is both implicitly encoded (i.e., $x =\lfloor {map(x,y)}\mbox{\%}\ C$) and explicitly encoded by the the values of variables $b_1 \ldots b_c$
 since it is easy to prove that $\psi_{boundaries}
 \wedge \psi_\uparrow$ forces $y = \oy_{map(x,y)}$.
 Finally, the conjuncts $\psi_{\exists} \wedge \psi_!$ ensure  that 
 each point in $n \in \{0, \ldots, N\}\}$, and thus, by means of $map$,
 any point in the grid, is associated with \emph{exactly} one tile,
 that is the unique tile variable  that belongs to $\cV([n,n])$.
 
For the aforementioned properties, if we consider the function 
 $f$ that maps a function  
 $\otile:\{0, \ldots, M\} \allowbreak \times \{ 0, \ldots, C\} \rightarrow \{0, \ldots, T\}$ in the model $\bfM = (M\cdot(C+1), \cV)$ 
 where for every $(x,y) \in \{0, \ldots, M\}\allowbreak  \times \{ 0, \ldots, C\}$
 we have  $t_i \in \cV([map(x,y), map(x,y)]) $ if and only if $\otile(x,y) = i$ and $\oy_{map(x,y)} = y$, it is easy to prove that $f$ is a bijection between the set of all such $\otile$ function, for every $M \in \bbN^+$,
 and the set of all finite models for $\psi_{\otile}$. 
In summary, the detailed description above shows that any model for $\psi_{\otile}$ is basically a way to represent a generic function $\otile:\{0, \ldots, M\}  \times \{ 0, \ldots, C\} \rightarrow \{0, \ldots, T\}$ and that, viceversa, each of such functions is represented by exactly one model of 
$\psi_{\otile}$. The next step is the encoding of the constraints
of Lemma~\ref{lem:finitecorridor} in $\mathsf{BA}_{hom}$
which allow to check whether there exists a function
$\otile$ that witnesses that $\cT$ is a positive instance.
Such  conditions, restricted to the finite case,
are imposed  by the following formulas:

\vspace{-0.6 cm}

\[\begin{array}{l}
\arraycellcomment{
\psi_{0,C} = \hsA \left(
	\left(\left(\pi \wedge \bigwedge\limits_{i=1}^C \neg b_i \right)\rightarrow t_0 \right)\wedge
	\left(\hspace{-0.1cm}\left(\pi \wedge \bigwedge\limits_{i=1}^C  b_i \right)\rightarrow t_T\hspace{-0.1cm}
  \right)\hspace{-0.1cm}
\right),\hspace{-0.1cm}
}{5.5cm}{ 
formula $\psi_{0,C} $ forces condition~\ref{prob:exptiling:topbot} of Problem~\ref{prob:exptiling}, that is,
the bottom tile of each column is $0$ and the top tile of each column is $T$;
}
\end{array}
\]
\[\begin{array}{l}
\arraycellcomment{
\psi_{\tileH} = \hsA \left(
  \pi \wedge \hsEA \neg \pi \rightarrow 
  \hsEA\left( \psi^{min}_=  \wedge \left(\bigvee\limits_{(i,j)\in \tileH}   (\hsEB t_i  \wedge \hsEA t_j )    \right) \right)
\right),
}{3.5cm}{ 
formula $\psi_{\tileH} $ forces condition~\ref{prob:exptiling:hor} of 
Problem~\ref{prob:exptiling}, that is, each pair of grid  points of
}\vspace{-0.0cm}\\ 
\mbox{\begin{tabular}{p{14.8cm}}
type $(x,y), (x+1,y)$ must be labelled with two tiles that are in the
$\tileH$ relation. This is done by taking for each point $n<N$ the minimal interval
$[n,n']$  with $n <n'$ and  $\oy_n = \oy_{n'}$; then, the $\tileH$ relation is forced 
between the pair of tile variables that hold over $[n,n]$ and $[n',n']$, respectively;
\end{tabular}
} %\\
\end{array}
\]
\[\begin{array}{l}
\arraycellcomment{
\psi^{min}_= = \psi^1_=  \wedge \hsAB \neg \psi^1_=,
}
{11.1cm}
{ formula $\psi^{min}_=$ holds over an interval $[n,n']$  if and only if $n <n'$, $\oy_n = \oy_{n'}$, and
does not exist $n<n''<n'$ such that $\oy_n = \oy_{n''}$. Let us notice that, 
for the constraints imposed by $\psi_{\otile}$ we have that
$n' - n = C + 1$ and thus, 
according to the definition  of $map$, we 
}\\ 
\mbox{\begin{tabular}{p{14.8cm}}
have $map^{-1}(n')=\allowbreak (\lfloor \frac{n}{C + 1} \rfloor + 1, n\ \mbox{\%}\ C) $;
then, $\psi^{min}_=$ holds on all and only those intervals whose endpoints represent horizontally adjacent points of the original grid; \end{tabular}}
%\\
\end{array}
\]
\[\begin{array}{l}
\arraycellcomment{
\psi_{\tileV} = \hsA\left( 
\hsAB \pi \wedge \bigvee\limits_{i=1}^{c} \neg b_i  \rightarrow\bigvee\limits_{(i,j)\in \tileV}   (\hsEB t_i  \wedge \hsEA t_j )
\right),
}{6.1cm}{ formula $\psi_{\tileV} $ forces condition~\ref{prob:exptiling:ver} of Problem~\ref{prob:exptiling}, that is,
each pair of grid points of type $(x,y), (x,y+1)$ must be labelled with two tiles that are
in the $\tileV$ relation. The constraint can be easily imposed 
since the encoding ensures 
  }\\ 
  \mbox{\begin{tabular}{p{14.8cm}}
that
vertical consecutive points in the grid corresponds to consecutive points in the model. The constraint 
is triggered on all the intervals of the type  $[n, n+1]$, with the exception of the of the ones with $\oy_n = C$.
The constraint imposes that  unique (thanks to $\psi_\exists\wedge \psi_!$)  pair of  tile variables $(t_i, t_j)$  with 
$(t_i) \in \cV([n,n])$ and $(t_j) \in \cV([n',n'])$ must  satisfy $(i,j) \in \tileV$.
%ones with $\oy_n = C$.
%The constraint imposes that  unique (thanks to $\psi_\exists\wedge \psi_!$)  pair of  tile variables $(t_i, t_j)$  with 
%$(t_i) \in \cV([n,n])$ and $(t_j) \in \cV([n',n'])$ must  satisfy $(i,j) \in \tileV$.
\end{tabular}
} 
 \end{array}
\]
\\
\[\begin{array}{l}
\arraycellcomment{
\psi_{prefix} = \! \!\! \!
\begin{array}{c}\hsEB\hsEA \left(p  \wedge  \bigwedge\limits_{i=1}^C  ( \hsEB(\pi \wedge \neg b_i) 
 \wedge \hsEA b_i )  \right) \wedge  \\ \hsA\left( p \wedge \pi  \rightarrow 
 \hsEA\left(\psi^1_= \wedge \hsAA  \neg \psi^1_= \wedge \bigwedge\limits_{i=0}^T (\hsEB t_i \leftrightarrow \hsA t_i)
  \right)\right)
  \end{array},
}{3.45cm}{ formula $\psi_{prefix}$ forces condition 4 of Lemma~\ref{lem:finitecorridor}, 
which 
imposes that there are two distinct columns in the grid
which are tiled identically and
}\\
\mbox{\begin{tabular}{p{14.8cm}}
one of such columns
is the last one.
 This is done by means of a propositional letter $p$. The first conjunct 
of formula $\psi_{prefix}$ imposes that there exists an interval $[n,n']$ in the model 
for which $p\in \cV([n,n'])$, $\oy_n=0$, and $\oy_{n'} = C$ (i.e., $p$ ``covers''
at least one column). Moreover, for the homogeneity assumption, 
we have that $p \in \cV([n'',n''])$  for every $n\leq n''\leq n'$.  The second conjunct imposes that 
for each $p$ labelled points $n$ there must exist a point $n'>n$ with $\oy_n= \oy_{n'}$
(this implicitly implies that $n$ is associated to a grid point which does not belong to the last column).
Moreover, formula $\hsAA  \neg \psi^1_=$ imposes that
 $n'$ must belong to the last column. Finally, it is required  that 
 there exists $0\leq i \leq T$ s.t.  $t_i \in \cV([n,n]) \cap \cV([n',n'])$.
\end{tabular}
}
\end{array}\]
 
\noindent Notice that in the above definitions the use of the $\hsEA$ operator enables us to deal with two key aspects: 
\begin{compactenum} 
\item we can predicate on all the intervals $[n,n']$
for any $n,n' \in \{0, \ldots, N\}$, whereas, by using the $\hsEB$
 operator alone,  we could predicate only on intervals of the form
  $[0, n]$;
 \item we can predicate on the ending point 
 of any current interval $[n,n']$, i.e., the interval $[n',n']$. 
 Such a feature is missing in the logic $\mathsf{BD}_{hom}$
 where we can predicate only on the beginning point of 
 any current interval. For instance, the logic $\mathsf{BD}_{hom}$
 cannot express properties like  $\psi^1_=$
 which checks whether the same  set of propositional letters 
 holds over the two ending points of an interval.
\end{compactenum}
 
Let us define now the formula $\varphi_{\cT}$ as 
$\varphi_{\cT}= \psi_{\otile} \wedge \psi_{0,C} \wedge \psi_{\tileH}\wedge \psi_{\tileV} \wedge \psi_{prefix}$. Since the models 
of  $\psi_{\otile}$ represent all and only the possible finite tiling functions for $\cT$ and 
$\psi_{0,C}$,$\psi_{\tileH}$, $\psi_{\tileV}$, $\psi_{prefix}$
select the subset of such functions/models where 
conditions \ref{prob:exptiling:topbot}, \ref{prob:exptiling:hor}, and
\ref{prob:exptiling:ver},  of Problem~\ref{prob:exptiling} together
with condition \ref{lem:finitecorridor} of Lemma~\ref{lem:finitecorridor} are fulfilled, we can prove the next result.

\begin{theorem}\label{thm:tilingiffsatisfiable}
Let $\cT = (T, \tileH,\tileV,C)$ be an instance of Problem~\ref{prob:exptiling}. Then, $\cT$ is a positive instance if and only if the $\mathsf{AB}_{hom}$ formula $\varphi_{\cT}$ is satisfiable over finite linear orders.
\end{theorem}

 It is easy to see that $\varphi_{\cT}$ 
may be generated in LOGSPACE. To this end, it suffices to observe that we may define a multitape Turing Machine that performs the reduction using just a constant amount of working tapes, each one holding either $\lceil\log_2 T\rceil$ bits or $c$ bits. 
From such an observation and Theorem~\ref{thm:tilingexpspacehard}, we obtain the same result of Section~\ref{sec:hardness}.

\thmabhomhard*
 
We conclude the section with some remarks that allow us to better understand how the homogeneity assumption affects the satisfiability problem of the considered $\mathsf{HS}$ fragments.
First of all, we observe that the complexity of the satisfiability problem for $\mathsf{AB}_{hom}$ over finite linear orders does not change if we replace it by full $\mathsf{AB}$, that is, if we remove the homogeneity assumption 
\cite{DBLP:journals/tcs/BresolinMMSS14}). Moreover, we would like to point out that the proof of the EXPSPACE-hardness of the satisfiability problem for $\mathsf{AB}_{hom}$, that is, the proof of Theorem~\ref{thm:abhomhard} to which this entire section is devoted, does not make use of the homogeneity assumption.
On the contrary, the homogeneity assumption marks a deep difference in $\mathsf{BDA}$: we proved that the satisfiability problem for $\mathsf{BDA}_{hom}$ 
 is decidable in exponential space, whereas the problem is known to be undecidable for full $\mathsf{BDA}$
 \cite{DBLP:journals/fuin/MarcinkowskiM14,DBLP:conf/icalp/MarcinkowskiMK10}. 
 As for model checking, the model checking problem  for $\mathsf{AB}_{hom}$ 
 over finite Kripke structures has been proved to be PSPACE-complete  \cite{DBLP:journals/tcs/BozzelliMMPS19},
 while here we proved that the satisfiability checking problem, over finite  linear orders, belongs to a higher complexity class, namely, \expspace. The tight complexity bound for the model checking problem over finite Kripke structures for $\mathsf{BDA}_{hom}$ is still open: we only know that for its three maximal proper fragments $\mathsf{AB}_{hom}$, $\mathsf{DA}_{hom}$, and  $\mathsf{BD}_{hom}$ it is PSPACE-complete \cite{DBLP:journals/tcs/BozzelliMMPS19,BMPS21}.
